# Supplementary material for: node2vec: Scalable Feature Learning for Networks
Source: arXiv:1607.00653 source file (2016-07-03)
Supplement: Supplementary file 1 [file 070appendix.tex]

\begin{itemize}
	\item ...
\end{itemize}
